# Supplementary material for: Group-Theoretic Upper Bounds on Reconstructability in Inverse Problems
Source: arXiv:2511.08995 source file (2026-09-02)
Supplement: Supplementary file 1 [file Supplemental_Material_arxiv.tex]

%===========================================================
% 補足資料（Supplemental Material）
% "Group-Theoretic Structure Governing Identifiability in Inverse Problems"
%===========================================================

\documentclass[aps,prl,twocolumn,notitlepage,superscriptaddress]{revtex4-2}
\usepackage{amsmath,amssymb,amsfonts,bm,graphicx}
\usepackage{physics}
\usepackage{booktabs}
\usepackage{hyperref}
\usepackage{siunitx}
\usepackage{here}
\usepackage{comment}
\usepackage[percent]{overpic}
\usepackage{placeins}
\begin{document}

\title{Supplemental Material\\
{Group-Theoretic Structure Governing Identifiability in Inverse Problems}}

\author{Isshin Arai}%
%\email{k078403@kansai-u.ac.jp}
\affiliation{1 Graduate School of Science and Engineering, Kansai University, Osaka, 564-8680, Japan}
\author{Tomoaki Itano}%
\affiliation{2 Department of Pure and Applied Physics, Faculty of Engineering Science, Kansai University, Osaka, 564-8680, Japan}

\date{\today}

%===========================================================
\maketitle

%===========================================================
\section{1. Identifiability Analysis}

\begin{table}[H]
\caption{Evolution of the identifiability limit with respect to the number of input pairs $N$. 
(a) Fundamental upper bound determined from group structure, 
(b) practical upper bound from the direct-sum mapping structure (main text), and 
(c) expected upper bound achievable by VGN (Fig.~\ref{fig:arch}).}
\label{tab:identifiability_appendix}
\begin{ruledtabular}
\begin{tabular}{c|ccc|c|ccc|c|ccc|c}
 & \multicolumn{4}{c|}{(a) Fundamental} & \multicolumn{4}{c|}{(b) Practical} & \multicolumn{4}{c}{(c) Expected} \\
$N$ & $V_0$ & $V_1$ & $V_2$ & Total & $V_0$ & $V_1$ & $V_2$ & Total & $V_0$ & $V_1$ & $V_2$ & Total \\ \hline
1 & 1 & 1 & 1 & 3 & 1 & 1 & 1 & 3 & 1 & 1 & 1 & 3 \\
2 & 1 & 3 & 5 & 9 & 1 & 2 & 2 & 5 & 1 & 3 & 3 & 7 \\
3 & 1 & 3 & 5 & 9 & 1 & 3 & 3 & 7 & 1 & 3 & 4 & 8 \\
4 & 1 & 3 & 5 & 9 & 1 & 3 & 4 & 8 & 1 & 3 & 5 & 9 \\
\end{tabular}
\end{ruledtabular}
\end{table}

The fundamental upper bound (a), derived from group structure, considers all combinations of the observation vectors 
$\{\mathbf{s}_i\}_{i=1}^N$ and $\{\dot{\mathbf{s}}_i\}_{i=1}^N$, 
corresponding to the total number of pairs ${}_{2N}C_2$. 
In this case, all representation components $(V_0,V_1,V_2)$ become, in principle, reconstructable at $N=2$.  
However, in practice, this theoretical bound is unattainable due to physical correlations and directional constraints in observation.

In this study, based on the physical mapping introduced in the main text (Eq.~(1)), 
each pair $(\mathbf{s}_i, \dot{\mathbf{s}}_i)$ is regarded as one independent unit of information, 
and effective upper limits are evaluated accordingly.  
Each input pair transforms under the action of the rotation group SO(3) as 
$V_1 \otimes V_1 = V_0 \oplus V_1 \oplus V_2$.  
For $N$ input pairs, the observation space expands as a direct sum 
$(V_0 \oplus V_1 \oplus V_2)^{\oplus N}$, 
and the corresponding degrees of freedom are shown as the practical upper bound (b).  
Furthermore, in the validation network (Fig.~\ref{fig:arch}), 
each input pair is integrated in a direct-sum manner and partially coupled through nonlinear layers (such as Gate and FullyConnectedTensorProduct modules \cite{Ge22}), 
which approximately realizes the expected product bound (c).

The limits (a–c) listed in Table~\ref{tab:identifiability_appendix} 
represent theoretical and predictive upper bounds determined by representation structure.  
In practice, these may not be fully achieved, depending on the input distribution or dominant physical systems.  
In particular, when linear independence of the input vectors is degraded or the directional distribution is biased, 
the reconstructable components decrease.  
Thus, although (b) and (c) suggest that full reconstruction becomes theoretically possible at $N=4$ or $N=5$, 
the actual reconstruction performance is governed by both the group-representation structure 
and the dominant physical systems.  
The identifiability limits derived here are consistent with the reconstruction results presented in Sec.~5–6.
\FloatBarrier
%===========================================================
\section{2. Dataset Generation and Simulation Setup}

The training and test datasets were numerically generated based on the orientational dynamics of particles suspended in an incompressible flow.  
Their motion is governed by
\begin{equation}
    \dot{\vb{s}} = \vb{s} \times \bigl( \vb{s} \times (\nabla \vb{u}\cdot \vb{s}) \bigr),
    \tag{s.1}
    \label{eq:dynamics}
\end{equation}
where $\vb{s}\in S^2$ is the particle orientation vector and $\nabla \vb{u}$ is the local velocity-gradient tensor
\cite{Je1922, Got11}.
For each $\nabla \vb{u}$, Eq.~\eqref{eq:dynamics} was directly integrated numerically with a time step of $\Delta t=2^{-14}$ to obtain the corresponding $\dot{\vb{s}}$.  
A total of $M=100$ orientation vectors $\{ \vb{s}_i \}_{i=1}^{M}$ were distributed nearly isotropically over the unit sphere, 
and for each velocity-gradient tensor, $N$ randomly selected pairs $(\vb{s}_i,\dot{\vb{s}}_i)$ were used as input samples.

Velocity-gradient tensors were generated from three representative spherical Couette flow (SCF) configurations \cite{Go21, Arai24}:
\begin{itemize}
    \item Axisymmetric flow,
    \item Two-fold spiral state,
    \item Three-fold spiral state.
\end{itemize}
A total of $10^4$ samples were generated for each configuration, 
yielding $3\times 10^4$ velocity-gradient tensors in total.  
For each tensor, $100$ orientation samples were produced, resulting in $100\times 3\times 10^4$ orientation data in total.  
The dataset was split into 80\% for training and 20\% for validating.  
Additionally, test data from the four-fold spiral state were used, comprising 24,500 velocity-gradient samples located within the same horizontal plane.
\FloatBarrier
%===========================================================
\section{3. Evaluation Metrics}

The evaluation metrics used in the main text are defined as follows:
\begin{align*}
    \text{Normalized Mean Squared Error (nMSE)} &:=
    \frac{\sum_i (\hat{T}_i - T^{\text{true}}_i )^2}{\sum_i (T^{\text{true}}_i)^2}, \\
    \text{Relative Squared Error (RSE)} &:=
    \frac{(\hat{T}_i - T^{\text{true}}_i )^2}{(T^{\text{true}}_i)^2}, \\
    \text{Mean Covariance Error (CovErr)} &:= 
    \Big\langle \| \hat{T}^{\rm rot}_i - R_i \hat{T}_i R_i^\top \|_F \Big\rangle,
\end{align*}
where $\hat{T}_i$ is the estimated velocity-gradient tensor and $R_i$ is the rotation applied to the input.  
In addition, Frobenius-norm-based errors were used when appropriate.

\FloatBarrier
%===========================================================
\section{4. Model Architecture and Training Conditions}

The proposed model, the \textit{Velocity Gradient Network} (VGN), 
was implemented using the e3nn library~\cite{Ge22} to ensure SO(3)-equivariance.  
Each $\vb{s}$ and $\dot{\vb{s}}$ is represented as a vector-type feature $V_1$ (denoted as {\it{1o}} in e3nn notation) 
and transformed through tensor products and gate mechanisms while preserving equivariance.

Figure~\ref{fig:arch} shows the schematic architecture of VGN.  
Hyperparameter optimization was performed under the condition $N=4$ (Table~\ref{tab:hyper}), 
where batch size $B$, depth $D$, and number of hidden units $u$ were varied sequentially, 
and the validation MSE was compared.  
Although increasing $u$ further reduced the loss, we fixed $u=128$ since the focus of this work is 
not on performance optimization but on verifying the relationship between identifiability limit and the number of input pairs $N$.

\begin{figure}[!htbp]%[h]
    \centering
    \includegraphics[width=0.8\linewidth]{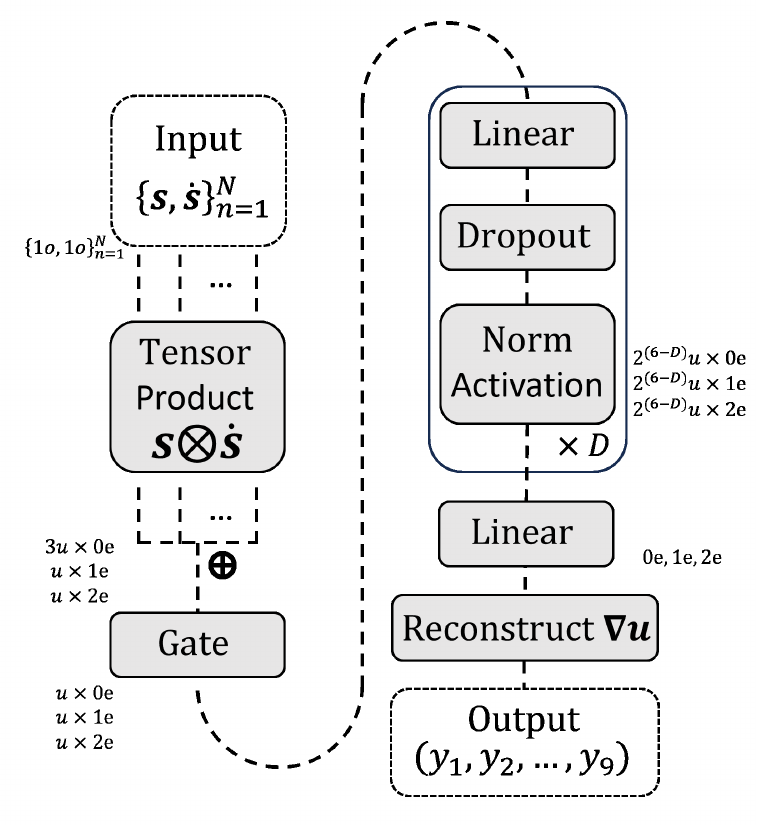}
    \caption{Schematic architecture of the Velocity Gradient Network (VGN).  
    Each input pair $(\vb{s}_i, \dot{\vb{s}}_i)$ is treated as an SO(3)-equivariant vector feature, 
    combined via tensor products, and mapped to the output tensor $\nabla \vb{u}$.}
    \label{fig:arch}
\end{figure}

\begin{table}[!htbp]%[h]
\caption{Hyperparameter search.}
\begin{ruledtabular}
\begin{tabular}{lcc}
Parameter & Search space & Final value \\ \hline
Batch size $B$ & 32, 64, 128 & 32 \\
Depth $D$ & 1, 2, 3 & 2 \\
Units $u$ & 16, 32, 64, 128, 256 & 128 \\
\end{tabular}
\end{ruledtabular}
\label{tab:hyper}
\end{table}
\FloatBarrier
%===========================================================
\section{5. Reconstruction Results}

This section presents the reconstruction results for the four-fold spiral state in SCF.  
For comparison, a standard multilayer perceptron (MLP) was also implemented 
under identical training conditions (batch size, Depth, and Units).
\paragraph{MLP.}
Each input pair $(\mathbf{s}_i, \dot{\mathbf{s}}_i)$ is concatenated and processed 
through several fully connected layers with tanh-activation and dropout 0.1 to output the reconstructed tensor.
\begin{table}[!htbp]%[t]
\caption{Comparison of estimation performance among models for $N=4$.}
\label{tab:comparison}
\begin{ruledtabular}
\begin{tabular}{lcc}
Metric & VGN & MLP\\ \hline
nMSE & $0.4027$ & $0.4816$ \\
MRSE & $0.4105$ & $0.5240$\\
CovErr & $2.52\times10^{-4}$ & $9.09\times10^{1}$ \\
\end{tabular}
\end{ruledtabular}
\end{table}
As shown in Table~\ref{tab:comparison}, compared with the MLP, which exhibits similar reconstruction errors (nMSE and MRSE),
the covariance error (CovErr) of the VGN is orders of magnitude smaller,  
demonstrating that the equivariant design stabilizes rotational variance in the estimation process.
Both the VGN and MLP were trained and validated under comparable conditions,
with hyperparameters adjusted to achieve stable convergence of the validation loss.
However, neither model was fully optimized for performance.

Table~\ref{tab:comparison_N} summarizes the reconstruction errors (nMSE, MRSE) 
for $N=3,4,5$ in each representation component.  
Figures~\ref{fig:hist_N3} and \ref{fig:hist_N5} show the corresponding RSE distributions.
As shown in Fig.~\ref{fig:hist_N3}, for $N=3$, 
the antisymmetric component $V_1$ (vorticity) is reconstructed accurately, 
while the symmetric traceless component $V_2$ (strain) exhibits a broad error distribution.  
In contrast, in Fig.~\ref{fig:hist_N5}, both $V_1$ and $V_2$ distributions shift toward lower errors, 
indicating partial reconstruction of $V_2$ as $N$ increases.  
These trends are consistent with the theoretical estimates of identifiable degrees of freedom in Table~\ref{tab:identifiability_appendix}, 
supporting that the proposed model quantitatively reflects the group-representation-based identifiability limit.

\begin{table}[!htbp]%[h]
\caption{Reconstruction errors for $V_1$ (rotation) and $V_2$ (strain) components.}
\label{tab:comparison_N}
\begin{ruledtabular}
\begin{tabular}{c|cc|cc|cc}
& \multicolumn{2}{c|}{$N=3$} & \multicolumn{2}{c|}{$N=4$} & \multicolumn{2}{c}{$N=5$}\\ 
Component & $V_1$ & $V_2$ & $V_1$ & $V_2$ & $V_1$ & $V_2$ \\ \hline
nMSE & $0.2716$ & $0.6805$ & $0.2096$ & $0.6183$ & $0.1641$ & $0.5495$\\
MRSE & $0.4239$ & $0.8108$ & $0.3112$ & $0.7939$ & $0.2736$ & $0.7627$\\
\end{tabular}
\end{ruledtabular}
\end{table}

% --- 図 1: N=3 ---
\begin{figure}[!htbp]%[h]
\centering
\begin{overpic}[width=0.9\columnwidth]{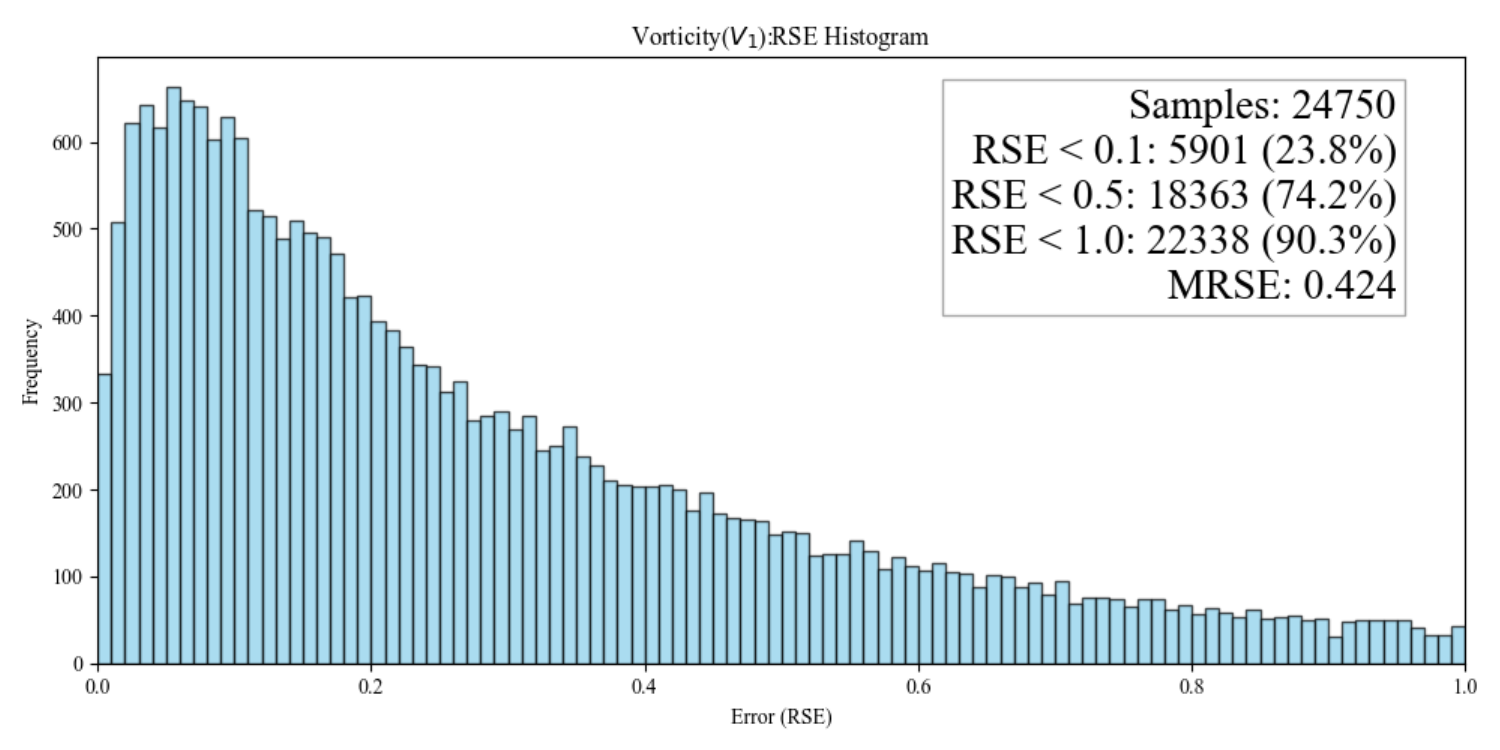}
  \put(5,48){\large (a)}
\end{overpic}
\vspace{2mm}
\begin{overpic}[width=0.9\columnwidth]{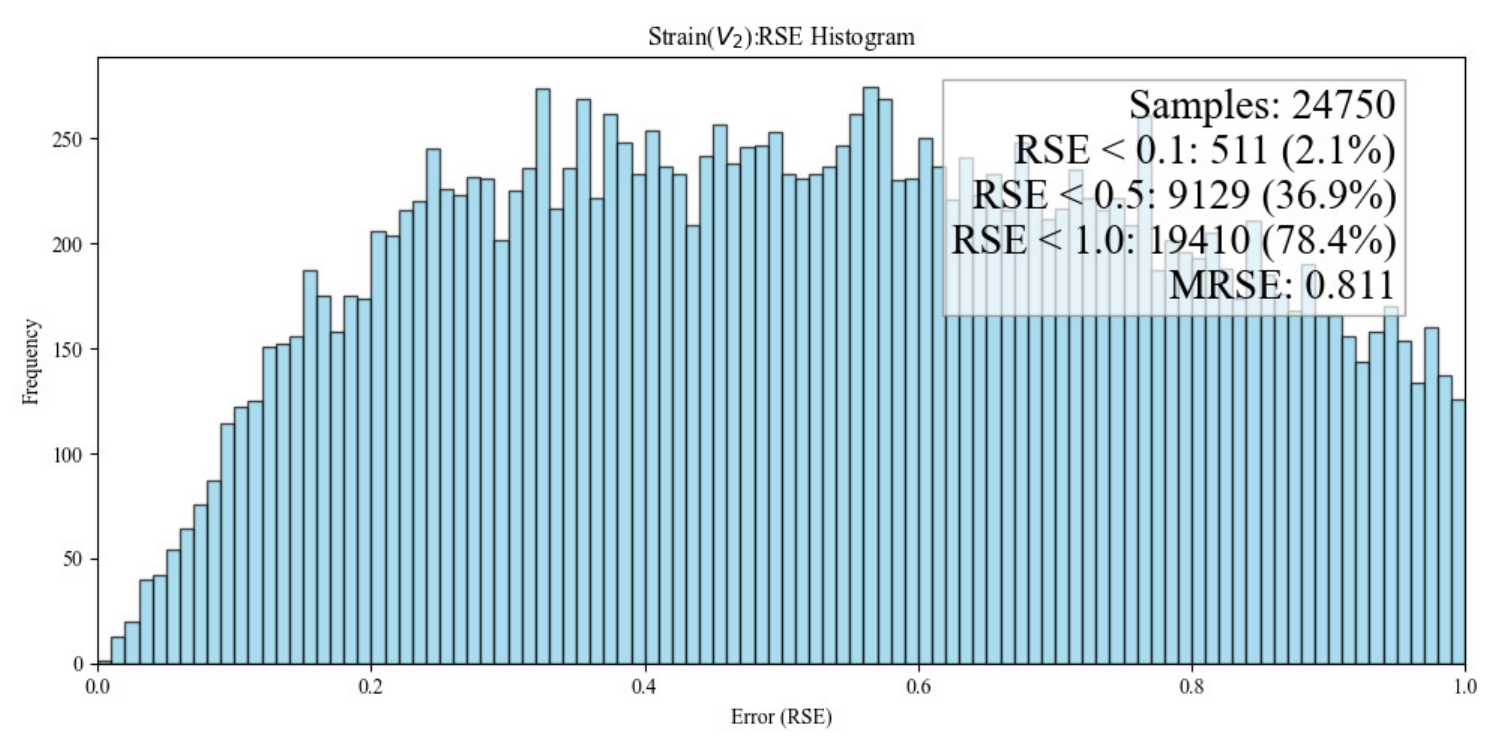}
  \put(5,48){\large (b)}
\end{overpic}
\caption{
RSE histograms for $N=3$.
(a) Vorticity component $V_1$, (b) strain component $V_2$.
The $V_1$ component shows high reconstruction accuracy, whereas the $V_2$ component exhibits a broad error distribution.
}

\label{fig:hist_N3}
\end{figure}

% --- 図 2: N=5 ---
\begin{figure}[!htbp]%[H]
\centering
\begin{overpic}[width=0.9\columnwidth]{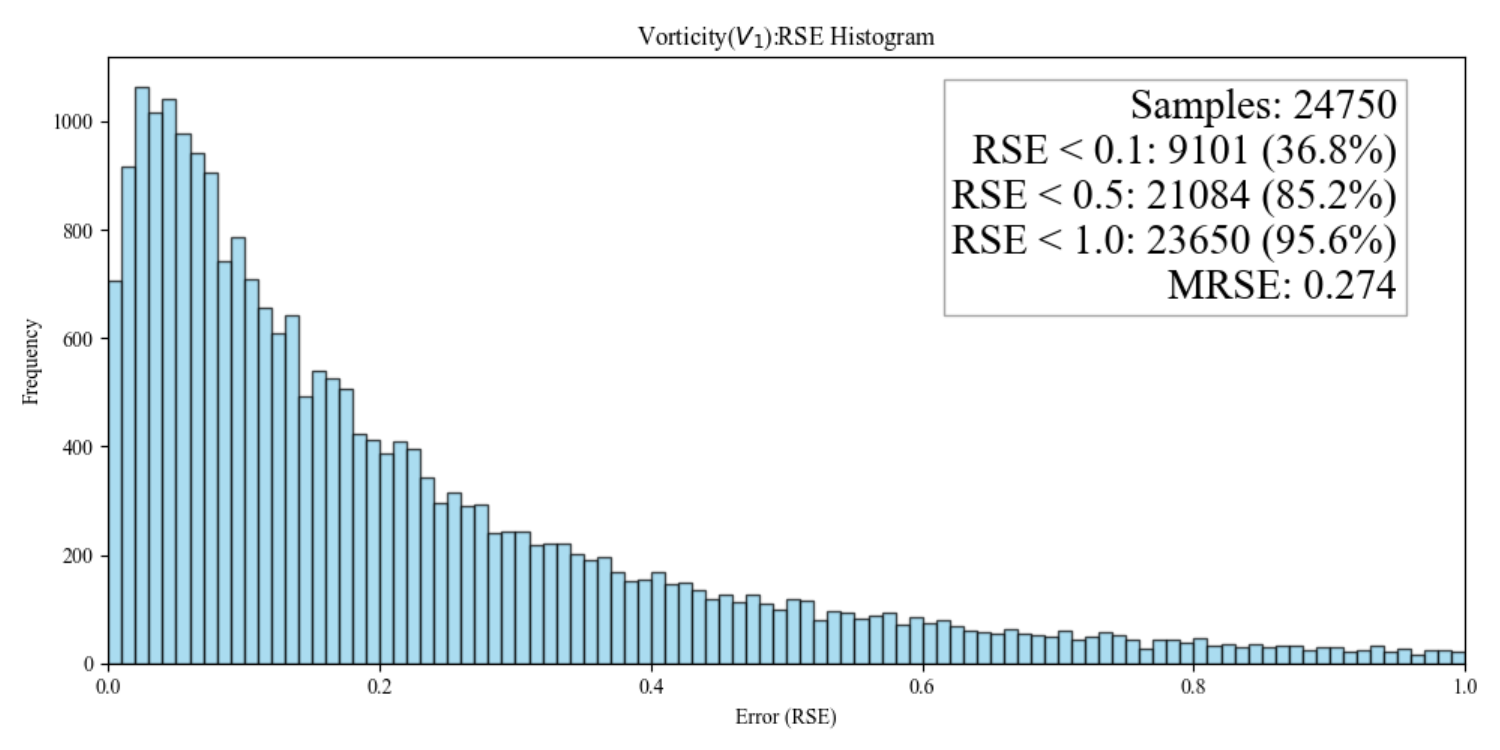}
  \put(5,48){\large (a)}
\end{overpic}
\vspace{2mm}
\begin{overpic}[width=0.9\columnwidth]{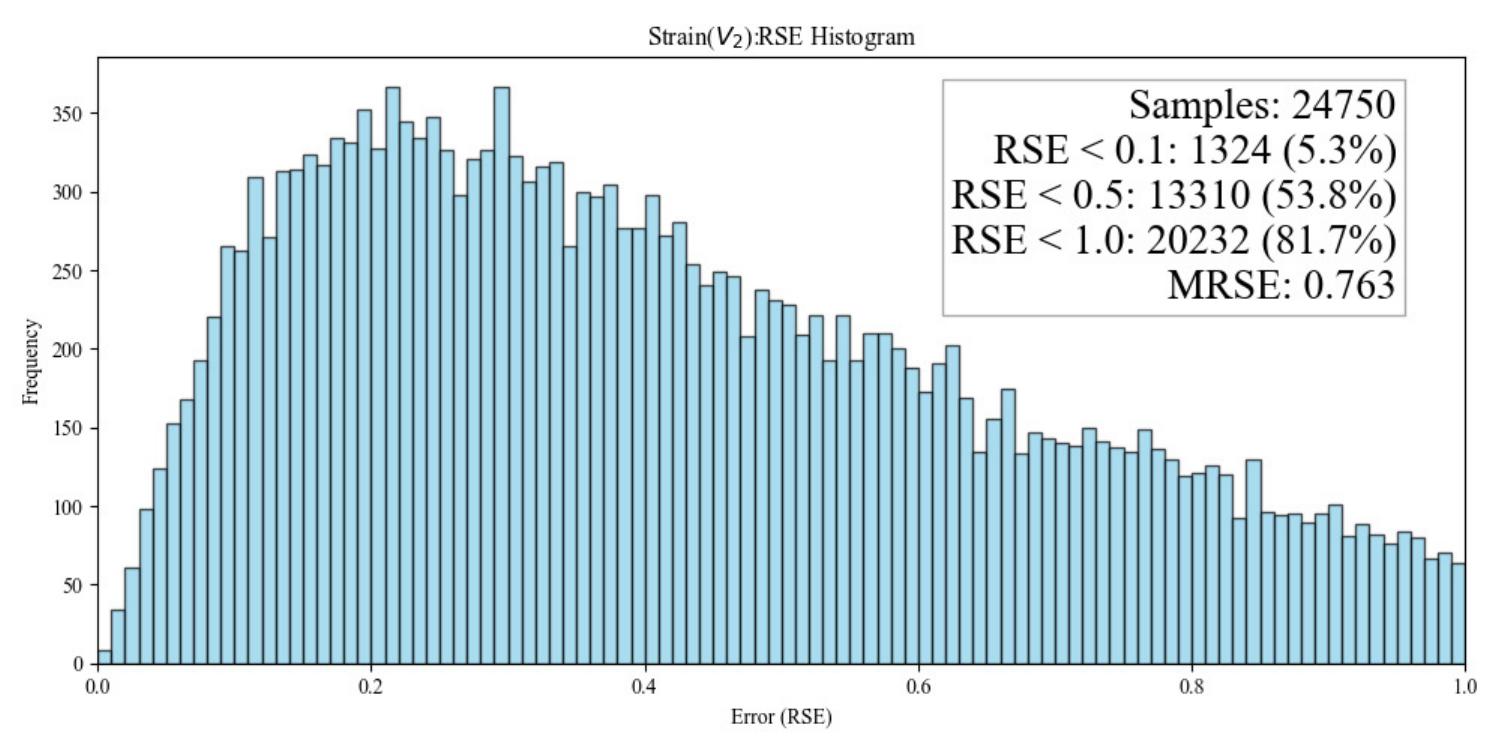}
  \put(5,48){\large (b)}
\end{overpic}
\caption{
RSE histograms for $N=5$.
(a) Vorticity component $V_1$, (b) strain component $V_2$.
The distribution of $V_2$ shifts toward lower error, indicating partial reconstruction progress.
}

\label{fig:hist_N5}
\end{figure}

\FloatBarrier
%===========================================================
\section{6. Visualization and Physical Interpretation of Velocity-Gradient Tensors}
%===========================================================

Figure~\ref{fig:velocitygrad_components} shows the Frobenius-norm spatial distributions of reconstructed velocity-gradient tensors for the $N=5$ case in the four-fold spiral state in SCF:  
(a) the total velocity-gradient tensor, (b) vorticity component $V_1$, and (c) strain component $V_2$, 
with the left and right panels showing the ground truth and VGN estimates, respectively.
The antisymmetric component $V_1$ (vorticity) exhibits a spatial pattern similar to the total tensor norm, 
whereas the symmetric component $V_2$ (strain) shows distinct spatial variation.  
This indicates that the dominant spatial mode of this dataset originates from the rotational component $V_1$, 
meaning that $V_1$ is the primarily excited physical mode.
\begin{figure}[htbp]%[h]
\centering
\includegraphics[width=0.9\columnwidth]{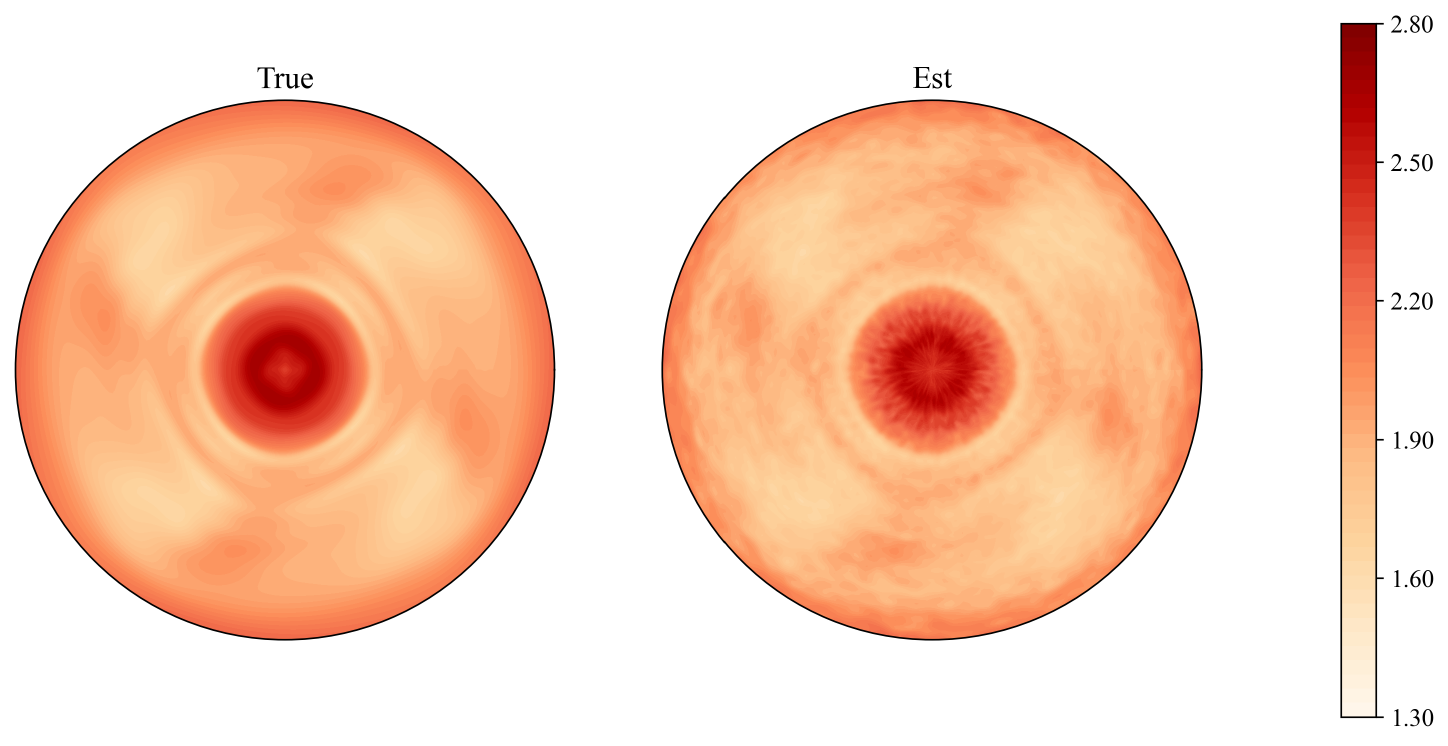}
\includegraphics[width=0.9\columnwidth]{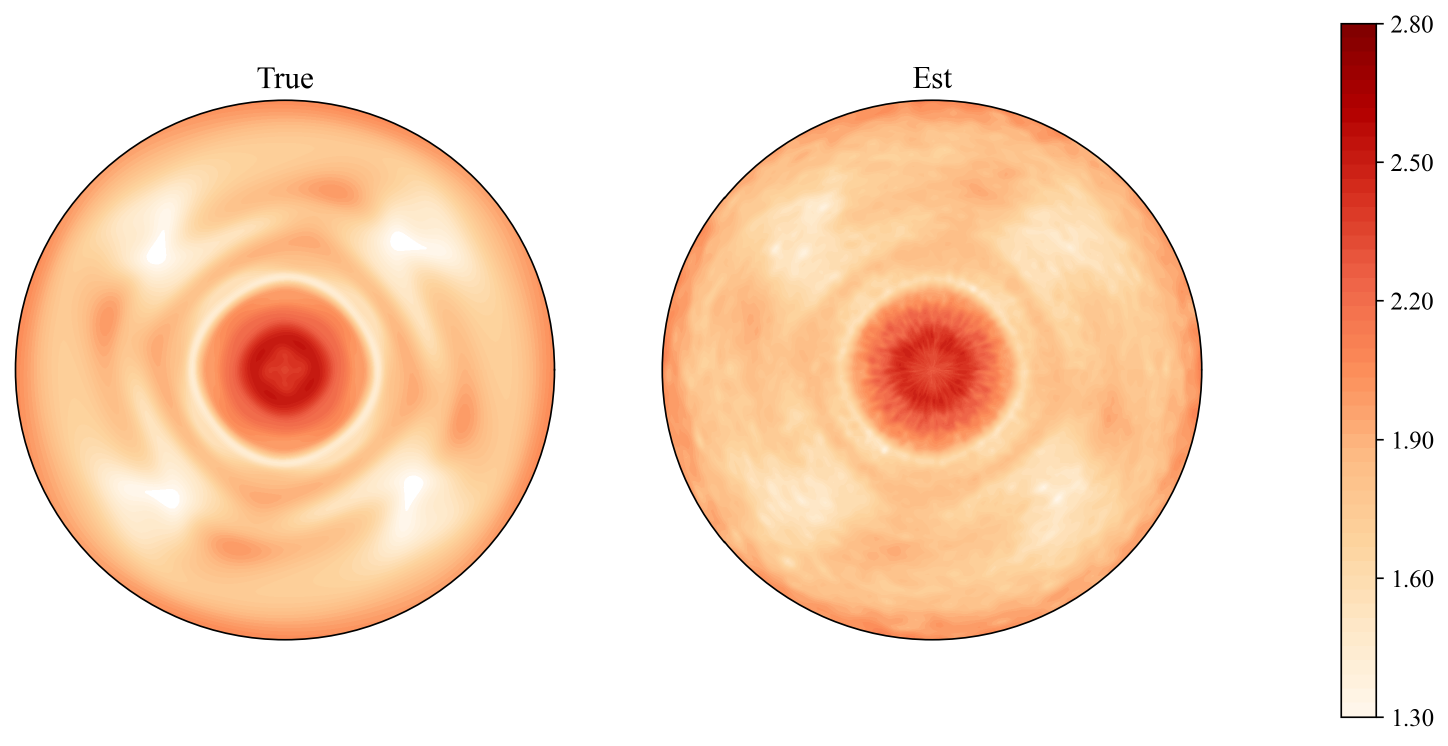}
\includegraphics[width=0.9\columnwidth]{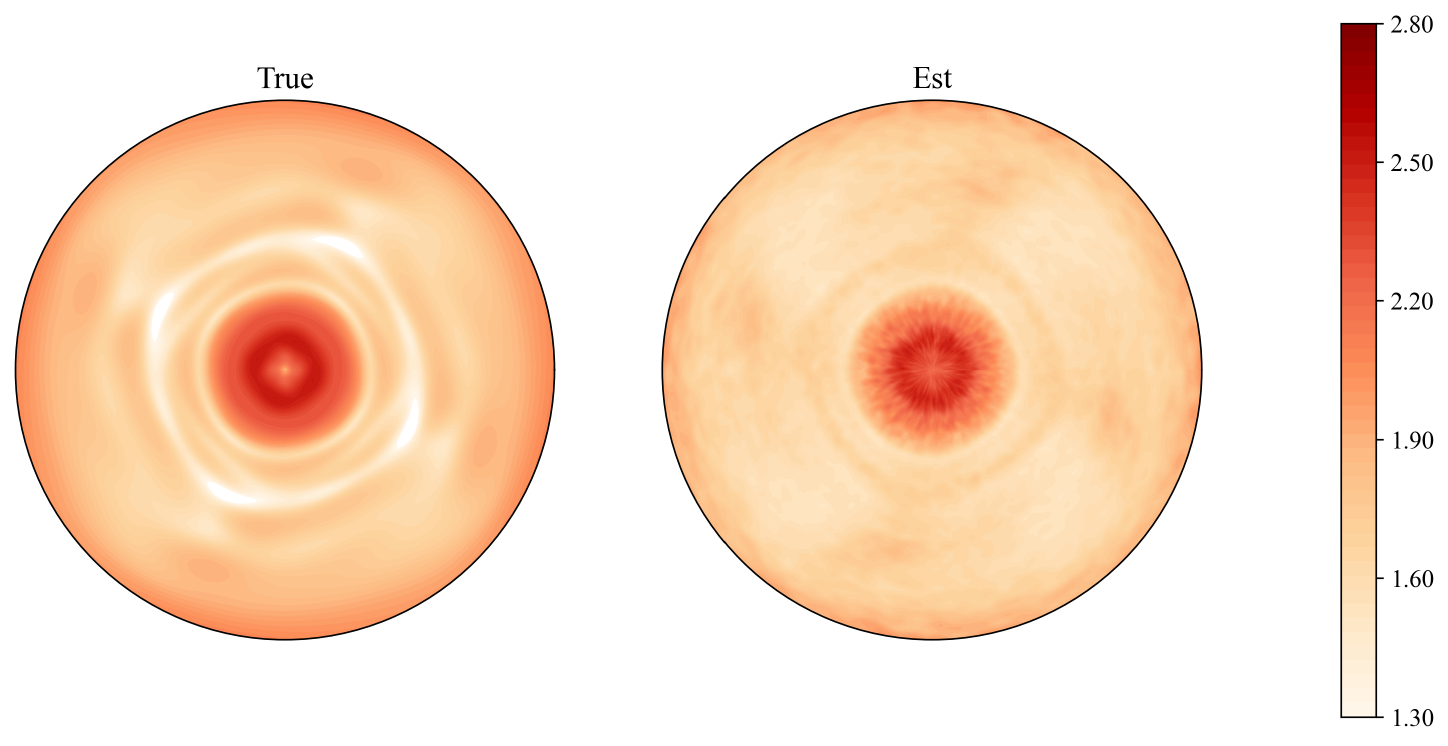}
\caption{
Comparison of Frobenius-norm ($\log_{10}$-scaled) spatial distributions of velocity-gradient tensors and their components ($N=5$).  
(a) Total tensor, (b) vorticity component $V_1$, and (c) strain component $V_2$.  
Left: ground truth; right: VGN estimate.}
\label{fig:velocitygrad_components}
\end{figure}
The analyzed system corresponds to particle orientation dynamics in SCF, 
where the inner sphere rotates while the outer sphere is stationary.  
The physical mapping Eq.~(\ref{eq:dynamics}) strongly depends on the $V_1$ component, 
hence the relatively large reconstruction error in $V_2$ arises not only from the theoretical identifiability limit 
but also from the dominance of $V_1$ as the physically excited hydrodynamic mode.
Finally, Fig.~\ref{fig:Frobenius Norm_N_5} shows the correlations and RSE distributions 
between true and reconstructed Frobenius norms of $V_1$ and $V_2$.  
Spatial variation is dominated by $V_1$, whose reconstruction accuracy is higher, 
while $V_2$ also shows improving agreement with the true values.

\begin{figure}[!htbp]%[h]
\centering
\begin{overpic}[width=0.9\columnwidth]{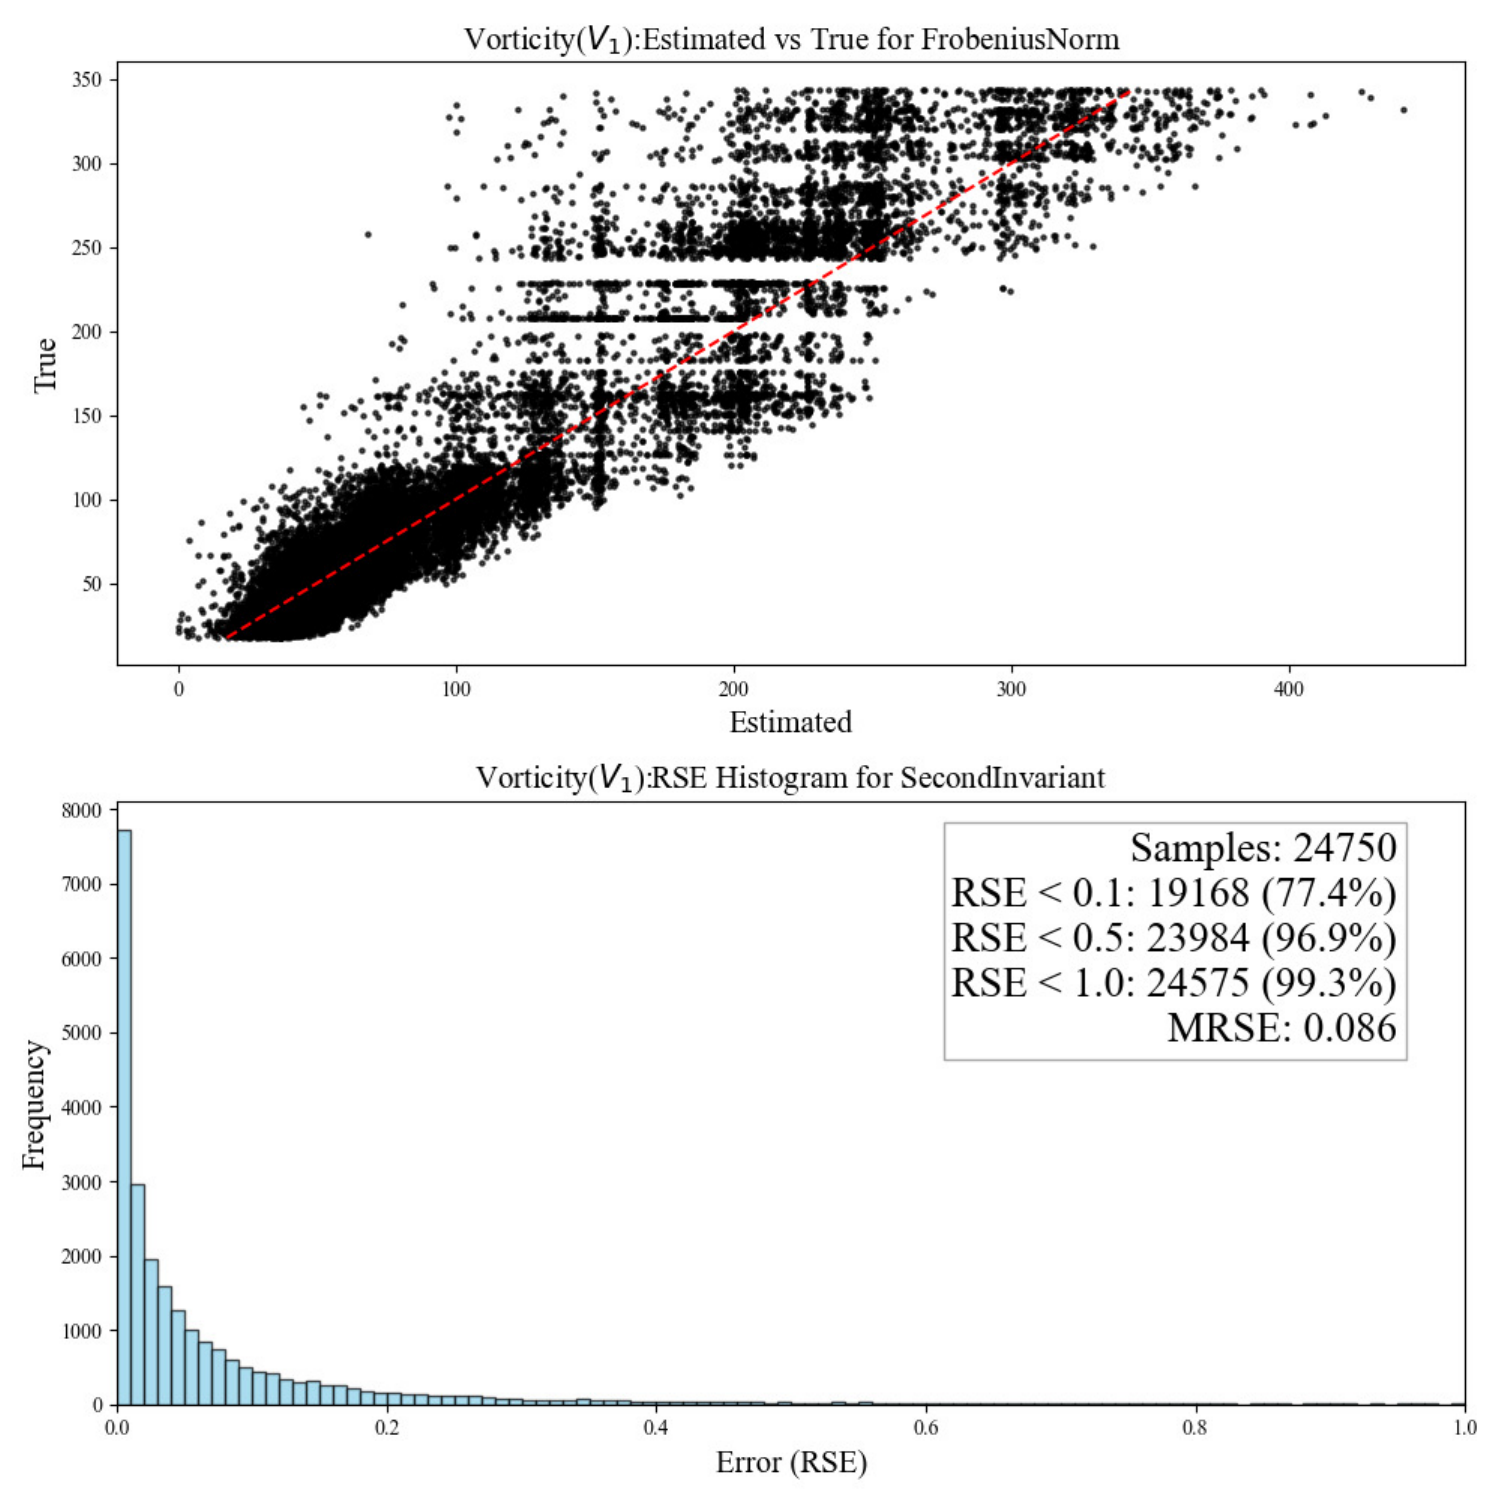}
  \put(5,100){\large (a)}
\end{overpic}
\vspace{2mm}
\begin{overpic}[width=0.9\columnwidth]{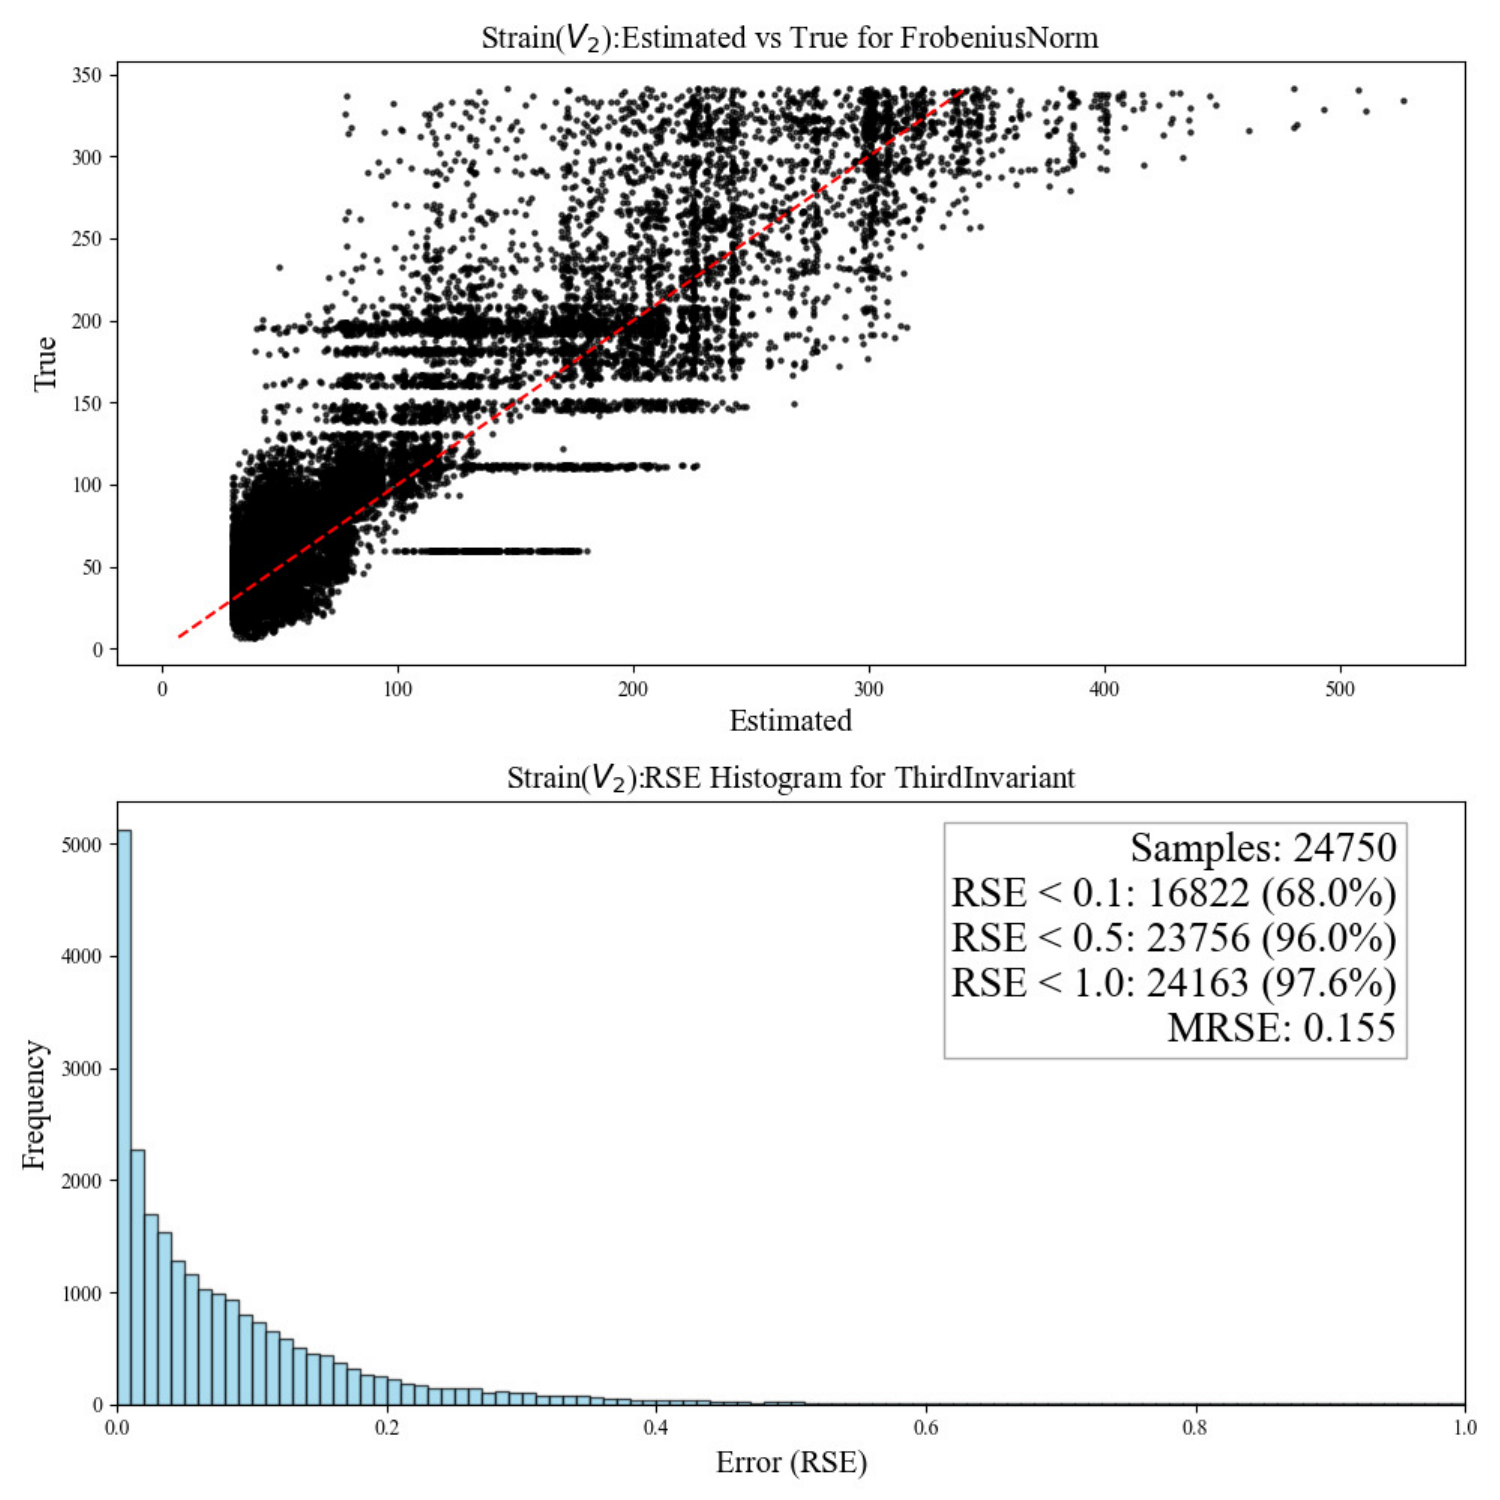}
  \put(5,100){\large (b)}
\end{overpic}
\caption{
Relationship between the true and predicted Frobenius norms of the velocity-gradient tensor components, and their RSE distributions ($N=5$).
(a) Vorticity component $V_1$, (b) strain component $V_2$.
Top panels show the correlation between true and predicted values, and bottom panels show the RSE histograms.
}
\label{fig:Frobenius Norm_N_5}
\end{figure}

\FloatBarrier
%===========================================================
\section{7. Noise Robustness Analysis}

Gaussian noise with mean 0 and standard deviation $\sigma$ was added to the orientation vectors $\vb{s}_i$, 
and reconstruction performance of the $V_1$ component was evaluated.  
The resulting RSE distributions are shown in Figs.~\ref{fig:hist_analyze_noise} and \ref{fig:hist_vgn_noise}.
\begin{figure}[!htbp]%[H]
\centering
\begin{overpic}[width=0.9\columnwidth]{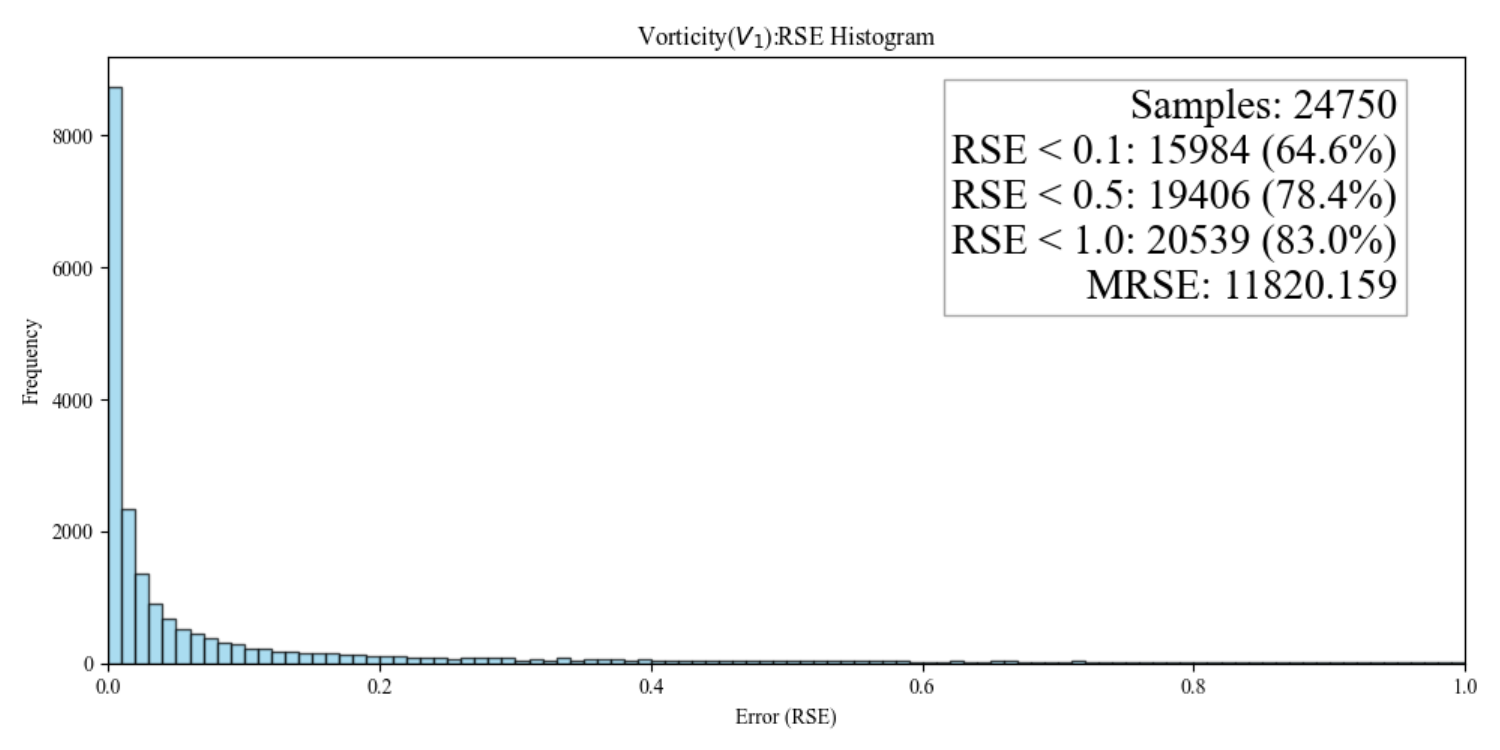}
  \put(5,48){\large (a) \small Gaussian noise $\sigma=10^{-4}$}
\end{overpic}
\vspace{2mm}
\begin{overpic}[width=0.9\columnwidth]{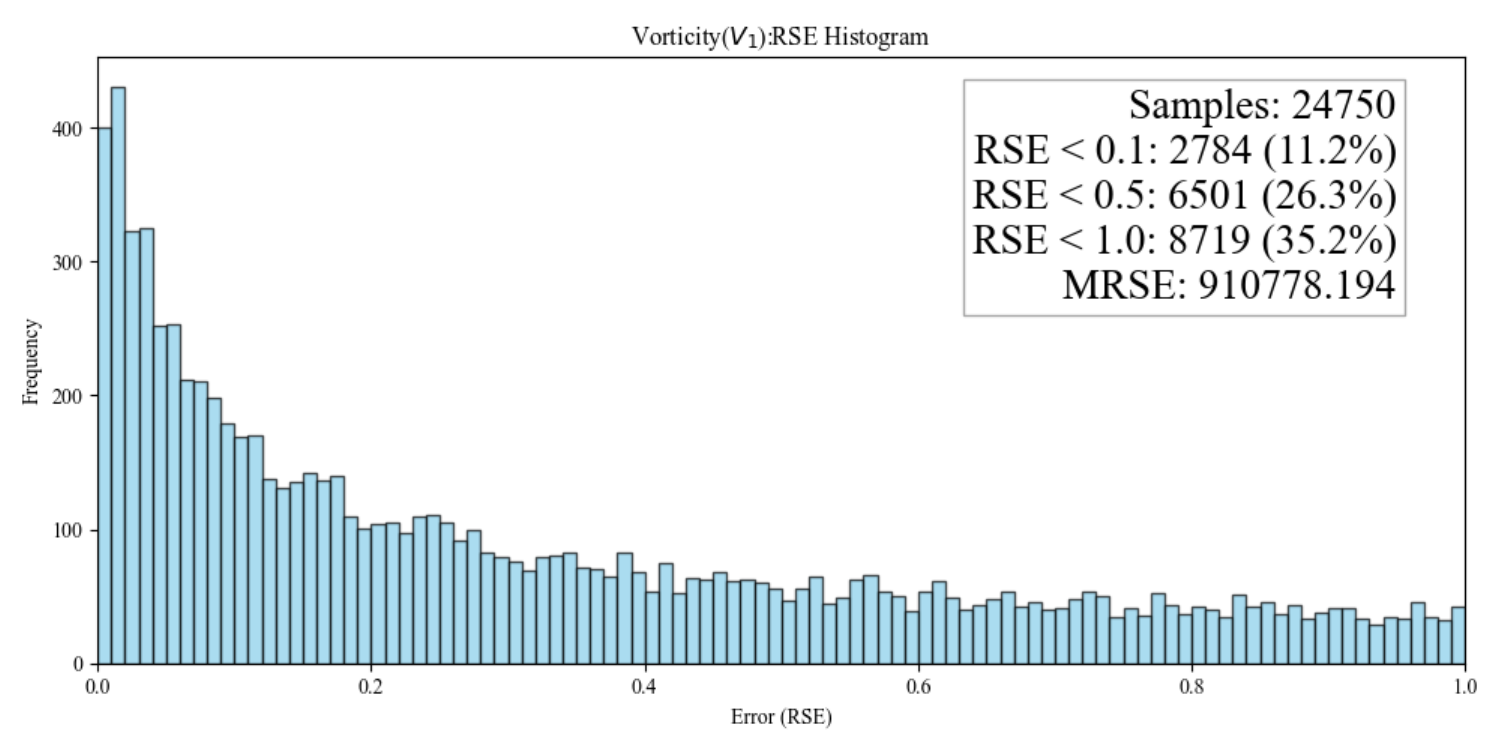}
  \put(5,48){\large (b) \small Gaussian noise $\sigma=10^{-3}$}
\end{overpic}
\caption{
RSE histograms of the vorticity component $V_1$ in the analytical reconstruction.
(a) $\sigma = 10^{-4}$, (b) $\sigma = 10^{-3}$.
The error distribution broadens as the noise level increases.
}
\label{fig:hist_analyze_noise}
\end{figure}

\begin{figure}[!htbp]%[H]
\centering
\begin{overpic}[width=0.9\columnwidth]{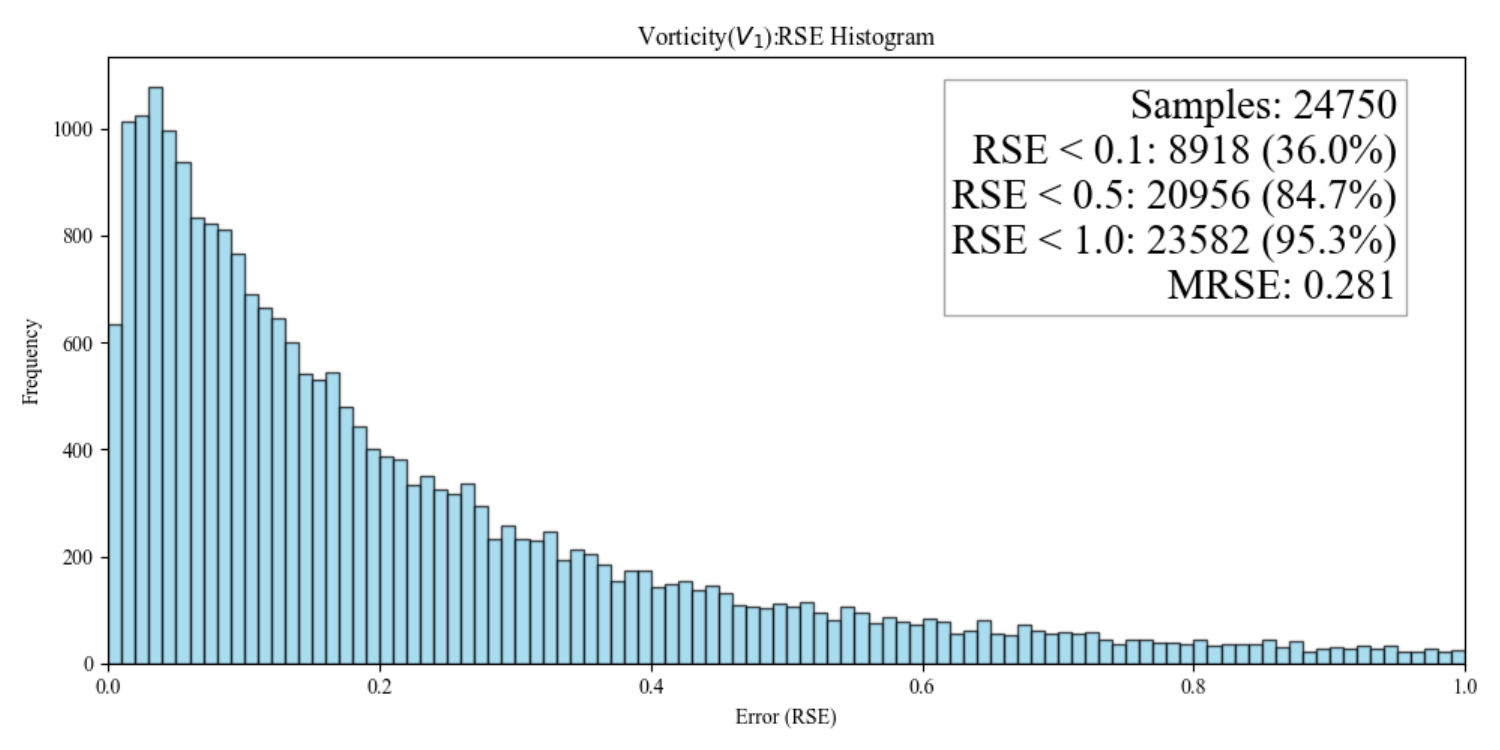}
  \put(5,48){\large (a) \small Gaussian noise $\sigma=10^{-4}$}
\end{overpic}
\vspace{2mm}
\begin{overpic}[width=0.9\columnwidth]{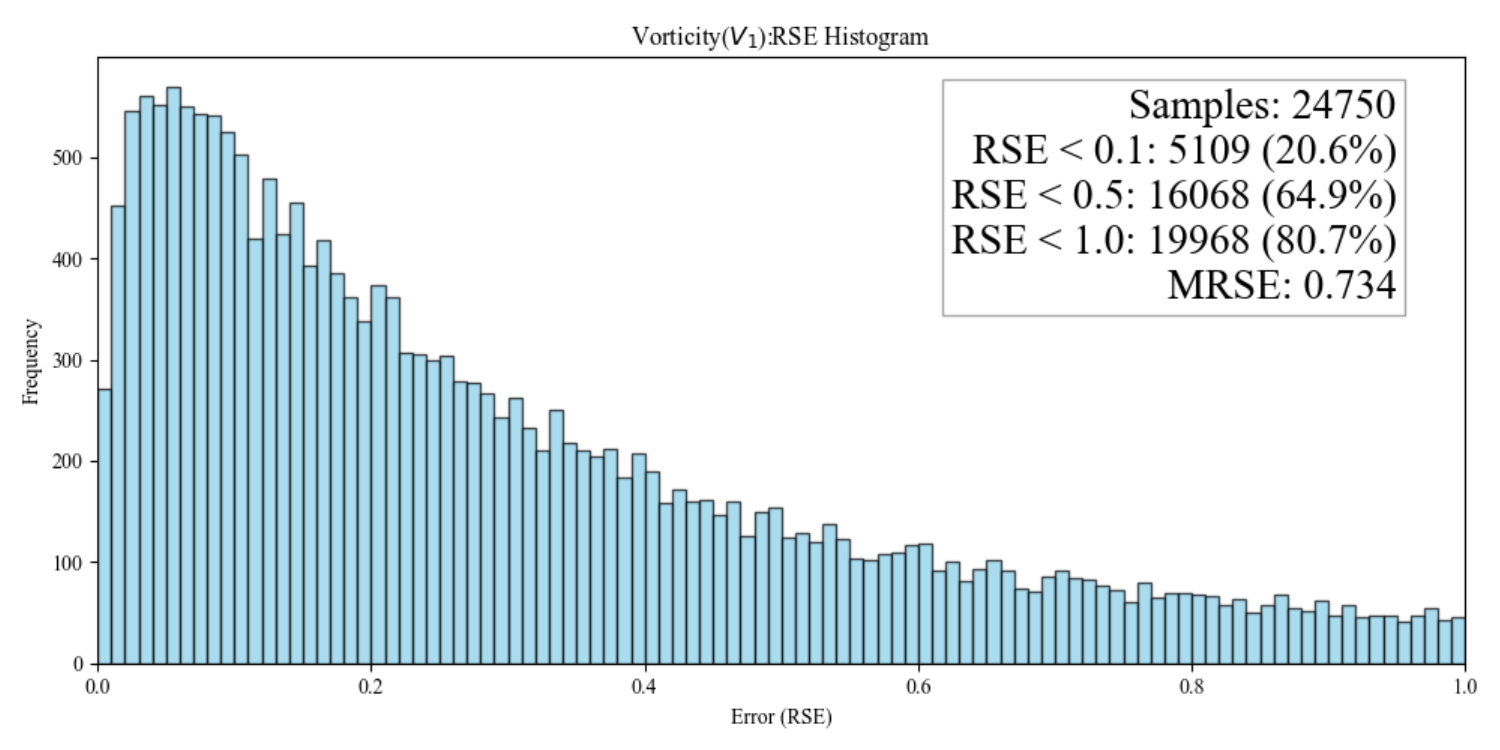}
  \put(5,48){\large (b) \small Gaussian noise $\sigma=10^{-3}$}
\end{overpic}
\caption{
RSE histograms of the vorticity component $V_1$ reconstructed by the VGN with $N=5$.
(a) $\sigma = 10^{-4}$, (b) $\sigma = 10^{-3}$.
High accuracy is maintained even under noisy conditions.
}
\label{fig:hist_vgn_noise}
\end{figure}
Figure~\ref{fig:hist_analyze_noise} shows the noise dependence in analytic reconstruction.  
For $\sigma = 10^{-3}$, the ratio of samples with RSE $<1$ drops to $35.2\%$, indicating high sensitivity to noise.  
In contrast, as shown in Fig.~\ref{fig:hist_vgn_noise}, 
the VGN with $N=5$ maintains $80.7\%$ of samples with RSE $<1$ under the same noise condition, 
demonstrating that the equivariant mapping of VGN provides strong robustness to input noise.

\FloatBarrier
\bibliography{supplemental}

\end{document}
